# Supplementary material for: Back to the Familiar Future: Failure Recovery for VLA Policies via Pre-Imagined Milestone Selection
Source: arXiv:2606.09258 source file (2026-12-03)
Supplement: Supplementary file 1 [file _appendix.tex]

\clearpage
\section*{Appendix}
\setcounter{section}{0}

\section{B2FF Implementation Details}

\subsection{Inference Modes of the Frozen Foresight-Driven VLA}
\label{app:inference_modes}

B2FF assumes a frozen foresight-driven VLA policy $\pi_\theta$ with an explicit future-image
interface. Given an instruction $I$, a current observation $o_t$, a future-image subgoal $v_t$, and
a length-$L$ action chunk $a_t=a_{t:t+L-1}$, we use the policy in two modes:
\begin{equation}
\label{eq:app_inference_modes}
\begin{aligned}
    \pi_\theta(v_t,a_t \mid I,o_t)
    &\quad \text{joint subgoal--action generation}, \\
    \pi_\theta(a_t \mid I,o_t;\; v_t \leftarrow v^\star)
    &\quad \text{action-only denoising with a fixed image subgoal}.
\end{aligned}
\end{equation}
The first mode is used during nominal execution. The second mode is used during recovery:
B2FF clamps the future-image subgoal to the selected familiar milestone $v^\star$ and generates
only the action chunk from the actual current observation $o_t$.

All calls to $\pi_\theta$ use frozen VLA weights. B2FF does not update the visual tokenizer,
future-image generator, action denoiser, or any other VLA backbone component. The only learned
components introduced by B2FF are the recoverability-aware selector $F_\phi$ and, for the
online-triggered variant, the trigger detector.
%%%%%%%%%%%%%%%%%%%%%%%%%%%%%%%%%%%%%%%%%%%%%%%%%%%%%%%%%
\subsection{Familiar Future Bank and Candidate Construction}
\label{app:familiar_future_bank}

Before executing any robot action, B2FF constructs an initial familiar future bank from the clean
initial observation $o_0$. We set $\tilde v_0=o_0$ and recursively query the future-image marginal
of the frozen VLA:
\begin{equation}
\label{eq:app_bank}
    \tilde v_m \sim \pi_\theta(v \mid I,\tilde v_{m-1}),
    \qquad m=1,\ldots,M_0 .
\end{equation}
The initial bank is $B=\{\tilde v_1,\ldots,\tilde v_{M_0}\}$. In our main experiments, we use
$M_0=12$. No actions are executed during this imagination rollout, so the bank contains familiar
visual milestones imagined from the clean initial state rather than futures re-predicted from a
failed observation.

When recovery begins at chunk-level index $f$, B2FF forms a local candidate set using offset set
$\Delta=\{-1,0,+1,+2,+4\}$:
\begin{equation}
\label{eq:app_candidates}
    C_f =
    \{\tilde v_{f+\delta}
    \mid
    \delta\in\Delta,\;
    1\leq f+\delta\leq |B|
    \}.
\end{equation}
The negative offset allows rollback, the zero offset retries the estimated progress point, and the
positive offsets allow near-future or skip-ahead recovery.

If a requested upper-end candidate index exceeds the current bank length, we deterministically
extend the bank by continuing imagination from the last available bank image until the required
index exists. This tail extension is used only to complete the local candidate set near the end of the
initial bank. It does not query the VLA from the failed observation and does not execute actions.
Lower out-of-range indices are discarded.

For each episode, all recovery methods and selection-rule baselines use the same bank, including
any deterministic tail-extended milestones. Thus, performance differences come from which
milestone is selected, rather than from different sampled banks.
%%%%%%%%%%%%%%%%%%%%%%%%%%%%%%%%%%%%%%%%%%%%%%%%%%%%%%%%%

\subsection{B2FF Inference Algorithm}
\label{app:b2ff_algorithm}

\begin{algorithm}[H]
\caption{\textsc{B2FF} Inference}
\label{alg:b2ff_inference}
\begin{algorithmic}[1]
\Require Frozen VLA $\pi_\theta$, selector $F_\phi$, instruction $I$, initial observation $o_0$,
initial bank size $M_0$, offsets $\Delta$, recovery window $W$, action chunk length $L$, horizon $T$
\Ensure Executed trajectory

\State $\tilde v_0 \gets o_0$, \quad $B \gets \emptyset$

\For{$m=1,\ldots,M_0$}
    \State $\tilde v_m \sim \pi_\theta(v \mid I,\tilde v_{m-1})$
    \State Append $\tilde v_m$ to $B$
\EndFor

\State $\texttt{mode} \gets \textsc{Nominal}$, \quad $r \gets 0$

\For{$t=1,\ldots,T$}
    \State Observe $o_t,p_t$ and update history $H_t$

    \If{$\texttt{mode}=\textsc{Nominal}$ \textbf{and} \textsc{Trigger}$()$}
        \State $s^\dagger \gets \textsc{TriggerStep}()$
        \State $f \gets \left\lceil s^\dagger / L \right\rceil$
        \State $m_{\max} \gets \max_{\delta\in\Delta}(f+\delta)$

        \If{$m_{\max} > |B|$}
            \State $m_{\mathrm{old}} \gets |B|$
            \For{$m=m_{\mathrm{old}}+1,\ldots,m_{\max}$}
                \State $\tilde v_m \sim \pi_\theta(v \mid I,\tilde v_{m-1})$
                \State Append $\tilde v_m$ to $B$
            \EndFor
        \EndIf

        \State $C_f \gets
        \{\tilde v_{f+\delta}
        \mid
        \delta\in\Delta,\;
        1\leq f+\delta\leq |B|
        \}$

        \State $v^\star \gets
        \arg\max_{\tilde v\in C_f}
        F_\phi(\tilde v \mid o_t,H_t,C_f)$

        \State $\texttt{mode} \gets \textsc{Recovery}$, \quad $r \gets W$
    \EndIf

    \If{$\texttt{mode}=\textsc{Recovery}$}
        \State $a_t \sim \pi_\theta(a \mid I,o_t;\; v_t \leftarrow v^\star)$
        \State $r \gets r-1$
        \If{$r=0$}
            \State $\texttt{mode} \gets \textsc{Nominal}$
        \EndIf
    \Else
        \State $(\hat v_t,a_t) \sim \pi_\theta(v,a \mid I,o_t)$
    \EndIf

    \State Execute action chunk $a_t$
    \If{\textsc{Terminal}$()$}
        \State \textbf{break}
    \EndIf
\EndFor
\end{algorithmic}
\end{algorithm}

\noindent
The bank is initialized with $M_0=12$ milestones in the main experiments. If recovery requires
candidate indices beyond the current bank length, B2FF extends the bank by continuing the same
future-image generation process from the last available bank image. This extension does not query
the VLA from the failed observation and does not execute actions. \textsc{TriggerStep} returns the
injected perturbation time in controlled evaluation and the first detector threshold crossing in the
online-triggered variant. Since bank indices are chunk-level, a trigger between the third and fourth
chunks is mapped to $f=4$.
%%%%%%%%%%%%%%%%%%%%%%%%%%%%%%%%%%%%%%%%%%%%%%%%%%%%%

\subsection{Indexing and Recovery Conventions}
\label{app:indexing_conventions}

B2FF uses chunk-level indexing because each familiar milestone corresponds to one action-chunk
step of nominal progress. Let $L$ be the number of low-level actions in one chunk. If a trigger
occurs at low-level step $s^\dagger$, we map it to the chunk-level recovery index
\begin{equation}
\label{eq:app_chunk_index}
    f=\left\lceil \frac{s^\dagger}{L}\right\rceil .
\end{equation}
For example, a trigger between the third and fourth chunks is assigned to index $f=4$. This
convention anchors recovery to the next chunk-level milestone rather than to the previously
completed chunk.

The recovery window $W$ is also measured in chunks. Once $v^\star$ is selected, B2FF keeps it
fixed as the future-image subgoal for $W$ consecutive action-generation calls. After this window,
the policy returns to nominal joint subgoal--action generation unless another recovery trigger is
activated.

In controlled failure-injected evaluation, \textsc{Trigger} fires at the injected perturbation time. In
the online-triggered variant, \textsc{Trigger} fires at the first threshold crossing of the learned
proprioceptive detector. Candidate-wise rollouts are used only offline for selector training and
upper-bound analysis, not during test-time recovery.
%%%%%%%%%%%%%%%%%%%%%%%%%%%%%%%%%%%%%%%%%%%%%%%%%%%

\section{Recovery-Mode Entry and Online Trigger}
\subsection{Controlled Recovery Timing}
\label{app:controlled_recovery_timing}

In the failure-injected LIBERO benchmark, we use controlled recovery timing to isolate the effect
of milestone selection from the separate problem of failure detection. Specifically, each evaluation
episode contains a known injected perturbation time. In the controlled setting, B2FF enters recovery
mode at the chunk-level index corresponding to this perturbation time, using the indexing convention
defined in Sec.~\ref{app:indexing_conventions}. If the perturbation occurs between two chunk-level
decision steps, we assign the recovery entry index to the next chunk.

This controlled timing does not provide the method with the correct recovery milestone. It only
specifies when recovery mode begins. After entering recovery mode, B2FF still constructs the local
candidate set from the familiar future bank and selects
\[
    v^\star = \arg\max_{\tilde v\in C_f}
    F_\phi(\tilde v \mid o_f,H_f,C_f),
\]
using a single forward pass of the selector. Candidate-wise trial rollouts are not used during
test-time recovery.

The purpose of this setting is to evaluate whether a selected pre-imagined familiar milestone can
serve as a better recovery condition than failed-state re-planning, fixed-anchor rules, or visual-nearest
matching when the recovery entry point is held fixed across methods. Thus, differences between
methods in the controlled benchmark reflect the quality of the recovery-time visual condition rather
than differences in trigger detection accuracy.

We report the online-triggered variant separately. In that setting, the recovery entry point is not
given by the perturbation time; instead, it is estimated from proprioceptive history using the learned
detector described in Sec.~\ref{app:online_detector}. This separates two sources of error: whether
B2FF can select a useful familiar milestone once recovery begins, and whether the system can detect
the appropriate recovery time online.
%%%%%%%%%%%%%%%%%%%%%%%%%%%%%%%%%%%%%%%%%%%%%%%%%%%%
\subsection{Online Detector Implementation}
\subsection{Trigger Timing Metrics}
\subsection{Missed, Early, Late, and False Triggers}
\subsection{Repeated-Trigger Handling}

\section{Recoverability-Aware Selector Architecture}
\label{app:selector_architecture}

\subsection{Selector Inputs and Output}
\label{app:selector_inputs}

At recovery entry index $f$, the selector receives the current failure observation $o_f$, a recent
observation history $H_f$, and a local candidate milestone set $C_f$. We use up to four history
frames in the final model. The candidate set contains up to five familiar milestones corresponding
to the offsets
\[
    \Delta=\{-1,0,+1,+2,+4\},
\]
which we refer to as previous, current, near, mid, and far candidates.

For each candidate $c_i\in C_f$, the selector outputs a scalar recoverability logit
\[
    s_i = F_\phi(c_i \mid o_f,H_f,C_f).
\]
At test time, B2FF selects the valid candidate with the largest score and uses it as the fixed
future-image subgoal:
\[
    v^\star = \arg\max_{c_i\in C_f} s_i .
\]
The score $s_i$ is used as a ranking logit, not as a calibrated success probability.

The implementation stores candidate metadata such as candidate type and offset index for logging
and batching. These metadata fields are not used by the final selector forward pass and are not
embedded in the scoring model.
%%%%%%%%%%%%%%%%%%%%%%%%%%%%%%%%%%%%%%%%%%%%%%%%
\subsection{Frozen Visual Tokenizer and Proxy-VQ Features}
\label{app:frozen_visual_tokenizer}

The selector uses pre-tokenized visual tokens from the frozen Emu3/UD-VLA visual tokenizer. Each
frame contains two views: a full-view image with $25\times25=625$ visual tokens and a wrist-view
image with $10\times10=100$ visual tokens. Each valid visual token id is mapped through the frozen
Emu3 VQ codebook to a 4-dimensional embedding. The final proxy-VQ frame feature is the
concatenation of the codebook embeddings from both views:
\[
    z(x)\in\mathbb{R}^{(625+100)\times 4}
    \equiv
    \mathbb{R}^{2900}.
\]
Thus, every observation or candidate milestone is represented as a 2900-dimensional continuous
proxy-VQ feature.

The visual vocabulary size is 32768, and the VQ codebook is used as a frozen buffer. The padding
token id is 32768 and is handled as padding rather than as a valid codebook entry. No visual
tokenizer or VQ codebook parameters are updated during selector training.

The main selector uses these frame-level proxy-VQ features. Token-embedding mean pooling is
used only in non-proxy baselines and is not the feature path used by the final model.
%%%%%%%%%%%%%%%%%%%%%%%%%%%%%%%%%%%%%%%%%%%%%%%%%%
\subsection{Step and Pair Projectors}
\label{app:step_pair_projectors}

The proxy-VQ feature for each frame is first passed through a step projector:
\[
\begin{aligned}
    h_x
    &=
    g_{\mathrm{step}}(z(x)) \\
    &=
    \mathrm{GELU}
    \left(
    W_2\,
    \mathrm{GELU}
    \left(
    W_1\,\mathrm{LN}(z(x))
    \right)
    \right),
\end{aligned}
\]
where $z(x)\in\mathbb{R}^{2900}$, the intermediate dimension is 512, and the output dimension is
256. In implementation, this corresponds to
\[
    \mathrm{LayerNorm}(2900)
    \rightarrow
    \mathrm{Linear}(2900,512)
    \rightarrow
    \mathrm{GELU}
    \rightarrow
    \mathrm{Linear}(512,256)
    \rightarrow
    \mathrm{GELU}.
\]

The pair projector represents the relationship between the current failure observation and another
history or candidate frame. For a frame $x$, we concatenate only the projected observation feature
and the projected frame feature:
\[
    p_x =
    g_{\mathrm{pair}}([h_{o_f};h_x]).
\]
The final implementation does not use difference features $h_{o_f}-h_x$ or product features
$h_{o_f}\odot h_x$. The pair projector is
\[
    \mathrm{LayerNorm}(512)
    \rightarrow
    \mathrm{Linear}(512,512)
    \rightarrow
    \mathrm{GELU}
    \rightarrow
    \mathrm{Linear}(512,256)
    \rightarrow
    \mathrm{GELU}.
\]

During the final RL-style selector fine-tuning stage, the step projector is frozen. The pair projector
is updated with a reduced learning rate, set to $0.3\times$ the main selector learning rate.
%%%%%%%%%%%%%%%%%%%%%%%%%%%%%%%%%%%%%%%%%%%%%%%%%%
\subsection{Perceiver-Style Candidate-Context Attention}
\label{app:perceiver_attention}

The selector uses a Perceiver-style architecture to aggregate history context and compare candidate
milestones. All selector hidden states have dimension 256. The context encoder uses 16 learnable
latent slots, 8 attention heads, dropout 0.1, and an MLP ratio of 4.0, corresponding to a 1024-
dimensional feed-forward hidden layer.

The context memory is built from history pair tokens. Let
\[
    P_H = \{p_x \mid x\in H_f\}
\]
denote the pair features between the failure observation and recent history frames. If no history is
available, we use a fallback context token formed from the observation paired with itself. The
learned context latents $\Lambda_0\in\mathbb{R}^{16\times256}$ first cross-attend to the history
pair tokens and are then processed by two latent self-attention blocks:
\[
    \Lambda =
    \mathrm{SelfAttn}^{(2)}
    \left(
        \mathrm{CrossAttn}(\Lambda_0, P_H)
    \right).
\]

Candidate pair tokens are then processed by the candidate encoder. Let
\[
    Q_C = \{p_{c_i}\mid c_i\in C_f\}
\]
be the candidate pair tokens. The candidate encoder applies two blocks, each consisting of
candidate self-attention followed by cross-attention from candidates to the context latents:
\[
    Q_C \leftarrow
    \left[
        \mathrm{CrossAttn}
        \left(
            \mathrm{SelfAttn}(Q_C), \Lambda
        \right)
    \right]^{(2)}.
\]
This allows candidates to compare against one another while also attending to the recent recovery
context.

Invalid candidate slots are masked by the candidate slot mask. Before the final argmax, invalid
candidate logits are set to $-10^9$ so they cannot be selected.
%%%%%%%%%%%%%%%%%%%%%%%%%%%%%%%%%%%%%%%%%%%%%%
\subsection{MLP Scoring Head}
\label{app:scoring_head}

For each valid candidate, the Perceiver candidate encoder returns a final candidate representation
$r_i\in\mathbb{R}^{256}$. The actor scoring head is a scalar linear head applied after layer
normalization:
\[
    s_i = W_{\mathrm{score}}\,\mathrm{LN}(r_i) + b_{\mathrm{score}}.
\]
The resulting scalar $s_i$ is a recoverability logit used for ranking candidate milestones. During
inference, we select the valid candidate with the largest score. If multiple candidates receive exactly
the same score, PyTorch's \texttt{argmax} returns the first maximum entry. Under the default
candidate ordering, this tie-breaking favors earlier slots in the order previous, current, near, mid,
and far. Exact ties are rare in practice.
%%%%%%%%%%%%%%%%%%%%%%%%%%%%%%%%%%%%%%%%%%
\subsection{Architecture, Input, and Candidate Ablations}
\label{app:selector_arch_ablation}

We report additional selector ablations on failure-injected LIBERO-Object using the same
120-episode evaluation protocol as the main selector analysis. All variants use the same frozen VLA
backbone and the same B2FF recovery interface. We vary only the selector architecture, selector
inputs, or number of candidate milestones.

\paragraph{Architecture ablation.}
Table~\ref{tab:perceiver_ablation} compares the final Perceiver-style selector against simpler
candidate scoring architectures. The MLP-only variant scores each candidate independently. The
Concat MLP variant concatenates candidate and context features before scoring. The shared-context
variant builds a single context feature and scores each candidate against it. The full selector uses
Perceiver-style candidate-context attention, which gives the strongest recovery performance.

\begin{table}[t]
\centering
\caption{
Selector architecture ablation on failure-injected LIBERO-Object.
All variants are evaluated under the same 120-episode Object recovery protocol.
}
\label{tab:perceiver_ablation}
\begin{tabular}{lc}
\toprule
Variant & Success (\%) \\
\midrule
MLP only & 61.7 \\
Concat MLP & 62.5 \\
Shared context + candidate & 66.7 \\
Full Perceiver selector & 69.3 \\
\bottomrule
\end{tabular}
\end{table}

\paragraph{Input ablation.}
Table~\ref{tab:selector_input_ablation_full} ablates the information available to the selector. This
table follows the same reporting format as the main selector input analysis. Observation-only
scoring is substantially weaker, while adding candidate milestones gives a large gain. Recent history
further improves recovery by providing temporal context for the off-trajectory state.

\begin{table}[t]
\centering
\caption{
Selector input ablation on failure-injected LIBERO-Object.
The final model uses the current observation, candidate milestones, and four history frames.
}
\label{tab:selector_input_ablation_full}
\begin{tabular}{lccc|cccc}
\toprule
Variant & Obs. & Cand. & Hist. & Grip. & Obj. & Lay. & All \\
\midrule
Obs. only & \checkmark & -- & 0 & 50.0 & 55.0 & 47.5 & 50.8 \\
+ Cand. & \checkmark & \checkmark & 0 & 60.0 & 65.0 & 60.0 & 61.7 \\
+ 1 hist. & \checkmark & \checkmark & 1 & 62.5 & 70.0 & 60.0 & 64.2 \\
+ 3 hist. & \checkmark & \checkmark & 3 & 70.0 & 70.0 & 60.0 & 66.7 \\
B2FF & \checkmark & \checkmark & 4 & 67.5 & 72.5 & 67.5 & 69.3 \\
\bottomrule
\end{tabular}
\end{table}

\paragraph{Candidate-count ablation.}
Table~\ref{tab:candidate_count_ablation} varies the number of familiar milestones available to the
selector. Using too few candidates limits the recovery hypotheses available to B2FF. The final
five-candidate setting performs best among the evaluated variants, while expanding to six
candidates does not further improve performance.

\begin{table}[t]
\centering
\caption{
Candidate-count ablation on failure-injected LIBERO-Object.
The final five-candidate setting corresponds to the default offset set
$\Delta=\{-1,0,+1,+2,+4\}$.
}
\label{tab:candidate_count_ablation}
\begin{tabular}{lc}
\toprule
Variant & Success (\%) \\
\midrule
2 candidates & 58.3 \\
3 candidates & 59.2 \\
4 candidates & 60.0 \\
5 candidates, final & 69.3 \\
6 candidates, expanded & 65.8 \\
\bottomrule
\end{tabular}
\end{table}
%%%%%%%%%%%%%%%%%%%%%%%%%%%%%%%%%%%%%%%%%%

\section{Selector Training}
\subsection{Training Pipeline Overview}
%%%%%%%%%%%%%%%%%%%%%%%%%%%%%%%%%%%%%%%%%%%%%%%%%%%%
\subsection{Proxy Temporal Initialization}
\label{app:proxy_temporal_initialization}

Training the selector directly from frozen visual tokens is sample-inefficient, because the selector
must learn both task progress and recoverability from a limited number of counterfactual recovery
rollouts. We therefore initialize the selector projectors with a proxy temporal task before the
supervised warm-start and offline fine-tuning stages. Given a current observation and a candidate
future image, the proxy model learns to estimate their temporal distance. This produces a
progress-aware embedding space that supports comparison among candidate familiar milestones.

\paragraph{Dataset.}
We run the baseline VLA and collect successful episodes from four LIBERO suites:
LIBERO-10, LIBERO-Goal, LIBERO-Object, and LIBERO-Spatial. From these trajectories, we
extract observation--future-milestone pairs. For a pair indexed by steps $a$ and $b$, the image at
step $a$ is an actual observation, while the image at step $b$ is the future reconstruction generated
by the VLA. The temporal-gap label is
\[
    g = |b-a|.
\]
To reduce bias toward frequent temporal distances, we stratify samples across five gap buckets:
\[
    [1,20],\quad [21,40],\quad [41,80],\quad [81,160],\quad >160 .
\]
This yields 190{,}156 samples, which we split into 80\% training, 10\% validation, and 10\% test
sets.

\paragraph{Model.}
We use a frozen Emu3 VisionTokenizer and extract continuous pre-VQ visual features from two
camera views: the front camera at resolution $200\times200$ and the wrist camera at resolution
$80\times80$. The proxy model contains three trainable components. First, a step projector
$g_{\mathrm{step}}$ concatenates the two camera features and maps them to a 256-dimensional step
representation:
\[
    s_x =
    g_{\mathrm{step}}
    \left(
        \left[
        E_{\mathrm{front}}(x_{\mathrm{front}});
        E_{\mathrm{wrist}}(x_{\mathrm{wrist}})
        \right]
    \right)
    \in \mathbb{R}^{256}.
\]
The same step projector is applied to both the observation and the candidate future milestone.
Second, a pair projector maps the two step representations to a joint pair representation:
\[
    z_{ab} = g_{\mathrm{pair}}\left([s_a;s_b]\right).
\]
Third, an auxiliary gap head $g(\cdot)$ predicts 5-class logits over the temporal-gap buckets. After
proxy pre-training, we discard the gap head and retain the step and pair projectors for selector
feature construction.

\paragraph{Loss.}
We optimize a weighted combination of a time-contrastive triplet loss and a temporal-gap
classification loss:
\[
    L_{\mathrm{proxy}}
    =
    L_{\mathrm{TCN}}
    +
    \beta_{\mathrm{gap}} L_{\mathrm{gap}},
    \qquad
    \beta_{\mathrm{gap}}=0.3.
\]

For each anchor representation $s_a$, we sample a positive representation $s_p$ within 10 steps
and a negative representation $s_n$ beyond 100 steps in the same episode. Using cosine distance
\[
    d(u,v)
    =
    1 -
    \frac{u^\top v}{\|u\|_2\|v\|_2},
\]
the time-contrastive triplet loss is
\[
    L_{\mathrm{TCN}}
    =
    \max
    \left(
        0,\,
        d(s_a,s_p)
        -
        d(s_a,s_n)
        +
        \alpha
    \right),
    \qquad
    \alpha=0.2.
\]
This objective pulls temporally nearby frames together and pushes distant frames apart.

The gap head produces logits $g(z_{ab})\in\mathbb{R}^{5}$ over the five temporal-gap buckets.
Let $y\in\{0,\ldots,4\}$ denote the ground-truth bucket index. The temporal-gap classification loss
is
\[
    L_{\mathrm{gap}}
    =
    -\log
    \frac{
        \exp(g_y(z_{ab}))
    }{
        \sum_{k=0}^{4}\exp(g_k(z_{ab}))
    }.
\]

\paragraph{Optimization.}
We train the proxy model for 50 epochs using AdamW with learning rate $1\times10^{-3}$ and a
cosine annealing scheduler. The Emu3 VisionTokenizer remains frozen throughout this stage; only
the step projector, pair projector, and auxiliary gap head are optimized.

\paragraph{Proxy pre-training results.}
On the held-out test set, the best checkpoint achieves 94.79\% temporal-gap classification accuracy
and 99.16\% TCN ranking accuracy. We compute TCN ranking accuracy as the fraction of sampled
triplets for which the learned embedding ranks the positive closer to the anchor than the negative:
\[
    d(s_a,s_p) < d(s_a,s_n).
\]
These results indicate that the learned embedding preserves temporal order well enough to support
distance-based milestone comparison in the downstream recoverability-aware selector.
%%%%%%%%%%%%%%%%%%%%%%%%%%%%%%%%%%%%%%%%%%%%%%%%%%%%%%%
\subsection{Counterfactual Rollout Label Collection}
\label{app:counterfactual_rollout_label_collection}

After proxy temporal initialization, we collect offline counterfactual recovery labels for training the
recoverability-aware selector. Each training example is a \emph{recovery group}, defined by one
injected training failure context:
\[
    x_i = (o_f^i, H_f^i, C_f^i),
\]
where $o_f^i$ is the failure observation, $H_f^i$ is the recent observation history, and $C_f^i$ is the
local candidate set constructed from the familiar future bank.

For each candidate $c \in C_f^i$, we clamp the future-image subgoal to that candidate,
$v^\star=c$, and roll out the frozen VLA in action-only denoising mode:
\[
    a_t \sim \pi_\theta(a \mid I,o_t;\; v_t \leftarrow c).
\]
The resulting binary label is
\[
    y_{i,c}
    =
    \mathbf{1}\{\text{the rollout succeeds}\}.
\]
Thus, each recovery group contains candidate-wise labels:
\[
    \mathcal{G}_i =
    \{(c,y_{i,c}) \mid c\in C_f^i\}.
\]

In total, we collect 400 injected training failure contexts, corresponding to 400 recovery groups.
With the default offset set $\Delta=\{-1,0,+1,+2,+4\}$, each group contains at most five candidate
milestones. Therefore, the total number of candidate-wise counterfactual rollouts is
\[
    N_{\mathrm{cf}}
    =
    \sum_{i=1}^{400} |C_f^i|
    \leq 400 \times 5 = 2000 .
\]
The exact number can be slightly smaller when lower-bound candidate indices are invalid near the
beginning of a bank. Each valid candidate is evaluated once using a five-chunk recovery rollout.

These candidate-wise rollouts are used only offline for selector supervision and candidate-oracle
upper-bound analysis. They are never used during test-time recovery. At test time, B2FF performs
a single selector forward pass, chooses the highest-scoring candidate, fixes it as $v^\star$, and
executes the frozen VLA without trying alternative candidates.
%%%%%%%%%%%%%%%%%%%%%%%%%%%%%%%%%%%%%%%%%%%%%%%%%%%%%%%%%%%
\subsection{Supervised Warm-Start Objective}
\label{app:supervised_warm_start}

After collecting counterfactual recovery labels, we first train the selector with supervised
candidate-wise objectives before applying the offline RL-style fine-tuning stage. Each training
sample is a recovery group
\[
    \mathcal{G}_f=\{(c,y_c)\mid c\in C_f\},
\]
where $C_f$ is the local candidate set for failure context $f$, and
$y_c\in\{0,1\}$ indicates whether fixing candidate $c$ as the future-image subgoal leads to final
task success.

Given selector score $s_c=F_\phi(c\mid o_f,H_f,C_f)$ for candidate $c$, we use a candidate-wise
binary cross-entropy loss:
\begin{equation}
\label{eq:app_bce}
    L_{\mathrm{BCE}}
    =
    -\frac{1}{|C_f|}
    \sum_{c\in C_f}
    \left[
        y_c \log \sigma(s_c)
        +
        (1-y_c)\log(1-\sigma(s_c))
    \right].
\end{equation}
We use positive class weight 1.0.

We also use a grouped softmax ranking objective within each recovery group. Let
\[
    Y_f=\sum_{c\in C_f}y_c
\]
be the number of successful candidates in group $f$. When $Y_f>0$, we apply
\begin{equation}
\label{eq:app_group}
    L_{\mathrm{group}}
    =
    -
    \frac{1}{Y_f}
    \sum_{c\in C_f} y_c s_c
    +
    \log
    \sum_{c\in C_f}\exp(s_c).
\end{equation}
This term encourages all successful candidates in the same failure context to receive higher
normalized scores than failed candidates. Unlike a single-positive classification objective, it does
not force the model to choose an arbitrary positive when multiple milestones can recover the task.
For all-fail groups, where $Y_f=0$, we omit $L_{\mathrm{group}}$ and train only with the BCE term.

The supervised warm-start objective is
\begin{equation}
\label{eq:app_lsup}
    L_{\mathrm{sup}}
    =
    \lambda_{\mathrm{BCE}} L_{\mathrm{BCE}}
    +
    \lambda_{\mathrm{group}} L_{\mathrm{group}},
\end{equation}
with $\lambda_{\mathrm{BCE}}=1.0$ and $\lambda_{\mathrm{group}}=1.0$.

We train the supervised selector warm-start for 20 epochs using AdamW with learning rate
$3\times10^{-4}$, weight decay $10^{-4}$, batch size 16, gradient clipping at 1.0, gradient
accumulation 1, and bf16 automatic mixed precision. We use random seed 42. The validation
criterion is the top-1 success rate, denoted \texttt{val\_top1\_success\_rate}. After each epoch, we
save a new best checkpoint when \texttt{val\_top1\_success\_rate} is greater than or equal to the
best metric observed so far. The best supervised checkpoint is obtained at epoch 20 with validation
top-1 success rate 0.6857.

\begin{table}[t]
\centering
\caption{
Supervised warm-start hyperparameters. The warm-start stage trains the selector on
counterfactual recovery records using candidate-wise BCE and grouped softmax ranking.
}
\label{tab:supervised_warm_start_hparams}
\begin{tabular}{lc}
\toprule
Item & Value \\
\midrule
$\lambda_{\mathrm{BCE}}$ & 1.0 \\
$\lambda_{\mathrm{group}}$ & 1.0 \\
Positive class weight & 1.0 \\
Optimizer & AdamW \\
Learning rate & $3\times10^{-4}$ \\
Weight decay & $10^{-4}$ \\
Batch size & 16 \\
Epochs & 20 \\
Gradient clipping & 1.0 \\
Gradient accumulation & 1 \\
AMP & bf16 \\
Random seed & 42 \\
Validation criterion & \texttt{val\_top1\_success\_rate} \\
Checkpoint rule & Save if validation metric improves or ties best \\
Best supervised checkpoint & Epoch 20 \\
Best validation top-1 success & 0.6857 \\
\bottomrule
\end{tabular}
\end{table}
%%%%%%%%%%%%%%%%%%%%%%%%%%%%%%%%%%%%%%%%%%%%%
\subsection{One-Step Actor-Critic-Style Fine-Tuning}
\label{app:one_step_actor_critic}

We further refine the selector using an offline one-step actor-critic-style objective. Each recovery
context $(o_f,H_f,C_f)$ defines a small discrete action space, where each candidate $c\in C_f$ is
one possible recovery choice. Since the counterfactual rollout label records whether choosing $c$
succeeds, we use the final task success label as the one-step reward target:
\[
    r_c = y_c.
\]
We use final success as the reward source, with reward scale 1.0 and discount factor 0.99.

\paragraph{Critic heads.}
We attach two critic heads on top of the candidate representation $r_i$. Each critic is a linear head
\[
    Q_k(r_i) = \mathrm{Linear}_{k}(r_i), \qquad \mathrm{Linear}_{k}: \mathbb{R}^{256}\rightarrow \mathbb{R},
    \qquad k\in\{1,2\}.
\]
The two critics are trained with PyTorch \texttt{smooth\_l1\_loss}, i.e., Huber regression with
default threshold $\delta_H=1.0$:
\begin{equation}
\label{eq:app_lq}
    L_Q
    =
    \mathbb{E}
    \left[
        \frac{w_f}{|C_f|}
        \sum_{c\in C_f}
        \sum_{k=1}^{2}
        \mathrm{Huber}_{1.0}
        \left(
            Q_k(c\mid o_f,H_f,C_f)-y_c
        \right)
    \right].
\end{equation}
The critic loss weight is 1.0.

\paragraph{Group weighting.}
We use recovery-group weights to emphasize contexts where selecting the right candidate matters
most. The final run uses the following rule:
\[
w_f =
\begin{cases}
0.5, & \text{all candidates fail},\\
0.5, & \text{all candidates succeed},\\
1.5, & \text{hard mixed group},\\
1.0, & \text{otherwise}.
\end{cases}
\]
A hard mixed group is a group with at least one successful candidate, but no successful candidate
among the baseline local candidates with offsets $\delta\in\{-1,0,+1\}$. In other words, these are
contexts where the easy previous/current/near candidates do not recover the task, and the selector
must choose a farther or otherwise less obvious candidate.

\paragraph{Actor-style selector update.}
The selector scores define a categorical distribution over candidates:
\[
    \pi_\phi(c\mid o_f,H_f,C_f)
    =
    \mathrm{softmax}(s)_c.
\]
We update the selector with an actor-style objective:
\begin{equation}
\label{eq:app_lactor}
    L_{\mathrm{actor}}
    =
    \mathbb{E}
    \left[
        w_f
        \sum_{c\in C_f}
        \mathrm{softmax}(s)_c
        \left(
            \alpha
            \log \mathrm{softmax}(s)_c
            -
            \min_{k\in\{1,2\}}
            Q_k(c\mid o_f,H_f,C_f)
        \right)
    \right].
\end{equation}
The actor loss weight is 1.0. We use a learned temperature initialized to 0.05, with target entropy
scale 0.4 and temperature learning rate $3\times10^{-4}$. The best checkpoint has learned
temperature approximately 0.0416.

\paragraph{Positive-candidate behavior-cloning regularizer.}
To stabilize fine-tuning and preserve the supervised preference for successful recovery choices, we
add a behavior-cloning regularizer toward the best-reward candidate in each group. The final
fine-tuning objective is
\begin{equation}
\label{eq:app_lft}
    L_{\mathrm{ft}}
    =
    L_Q
    +
    L_{\mathrm{actor}}
    +
    \lambda_{\mathrm{BC}} L_{\mathrm{BC}},
\end{equation}
where $\lambda_{\mathrm{BC}}=0.5$. In our implementation, $L_{\mathrm{BC}}$ uses the best-reward
candidate as the BC target. This regularizer biases the selector toward candidates with observed
recovery success while the critic and actor terms refine the score distribution over the full candidate
set.

\paragraph{Optimization details.}
We fine-tune the selector for 8 epochs with 200 optimization steps per epoch, for a planned total of
1600 RL fine-tuning steps. We use AdamW with learning rate $10^{-4}$ for the main selector
parameters and a smaller learning rate of $3\times10^{-5}$ for the pair projector, corresponding to
a 0.3 multiplier. The batch size is 16, weight decay is $10^{-4}$, gradient clipping is 1.0, and the
target update coefficient is $\tau=0.01$. We use random seed 42.

We do not use patience-based early stopping in the final RL run. Instead, training is run for the full
8 epochs, and the checkpoint with the best validation top-1 success rate is saved as
\texttt{best.ckpt}. The best checkpoint is selected at epoch 3, step 600.
%%%%%%%%%%%%%%%%%%%%%%%%%%%%%%%%%%%%%%%%%%%%
\subsection{Selector Training Ablations}
\label{app:selector_training_ablations}

We ablate the selector training pipeline on failure-injected LIBERO-Object. All variants use the
same frozen VLA, familiar future bank construction, candidate offset set, and recovery interface.
They differ only in how the selector is initialized or fine-tuned. Table~\ref{tab:selector_training_ablation_app}
shows that the full training pipeline improves overall success from 63.3\% for scratch supervised
training to 69.3\%. The intermediate variants provide partial gains but do not match the full
fine-tuning objective, indicating that positive-candidate BC alone is insufficient without the more
stable Huber critic regression and lower-entropy actor update.

\paragraph{Training objective ablation.}
Table~\ref{tab:selector_training_ablation_app} compares five variants. \emph{Scratch sup.} trains
the selector from counterfactual labels without proxy temporal initialization. \emph{Proxy sup.}
adds proxy temporal initialization but stops after supervised warm-start. \emph{Weak RL} applies
a reduced-strength one-step actor-style update. \emph{RL + Pos. BC} adds behavior-cloning
regularization toward positive candidates. The full B2FF selector combines proxy initialization,
supervised warm-start, Huber critic regression, a lower-entropy actor update, and positive-candidate
BC regularization.

\begin{table}[t]
\centering
\caption{
Selector training objective ablation on failure-injected LIBERO-Object. FT denotes the final
fine-tuning stage. Values are task success rates (\%).
}
\label{tab:selector_training_ablation_app}
\begin{tabular}{lccc|cccc}
\toprule
Variant & Proxy & Sup. & FT & Grip. & Obj. & Lay. & All \\
\midrule
Scratch sup. & -- & \checkmark & -- & 62.5 & 67.5 & 60.0 & 63.3 \\
Proxy sup. & \checkmark & \checkmark & -- & 67.5 & 67.5 & 60.0 & 65.0 \\
Weak RL & \checkmark & \checkmark & weak RL & 67.5 & 70.0 & 60.0 & 65.8 \\
RL + Pos. BC & \checkmark & \checkmark & pos. BC & 67.5 & 70.0 & 60.0 & 65.8 \\
B2FF & \checkmark & \checkmark & Huber+LE+BC & 67.5 & 72.5 & 67.5 & 69.3 \\
\bottomrule
\end{tabular}
\end{table}

The full B2FF objective performs best overall, improving from 63.3\% for scratch supervised
training to 69.3\%. The intermediate variants provide partial gains but do not match the full
fine-tuning objective, indicating that positive-candidate BC alone is insufficient without the more
stable Huber critic regression and lower-entropy actor update.

\paragraph{Selector input ablation.}
Table~\ref{tab:selector_input_ablation_app} studies which inputs are needed for recoverability-aware
milestone scoring. Observation-only scoring is weak because it cannot compare the failed state
against candidate familiar futures. Adding candidate milestones substantially improves performance.
Adding recent history further improves the selector, indicating that short-term visual context helps
determine which familiar milestone is reachable from the current off-trajectory state.

\begin{table}[t]
\centering
\caption{
Selector input ablation on failure-injected LIBERO-Object. Hist. denotes the number of recent
history frames used by the selector. Values are task success rates (\%).
}
\label{tab:selector_input_ablation_app}
\begin{tabular}{lccc|cccc}
\toprule
Variant & Obs. & Cand. & Hist. & Grip. & Obj. & Lay. & All \\
\midrule
Obs. only & \checkmark & -- & 0 & 50.0 & 55.0 & 47.5 & 50.8 \\
+ Cand. & \checkmark & \checkmark & 0 & 60.0 & 65.0 & 60.0 & 61.7 \\
+ 1 hist. & \checkmark & \checkmark & 1 & 62.5 & 70.0 & 60.0 & 64.2 \\
+ 3 hist. & \checkmark & \checkmark & 3 & 70.0 & 70.0 & 60.0 & 66.7 \\
B2FF & \checkmark & \checkmark & 4 & 67.5 & 72.5 & 67.5 & 69.3 \\
\bottomrule
\end{tabular}
\end{table}

These ablations show that recoverability-aware selection benefits from both candidate-relative
comparison and recent observation history. This supports the design choice of scoring each familiar
milestone under the full recovery context $(o_f,H_f,C_f)$ rather than using only the failed
observation or a fixed progress rule.

\paragraph{Optional all-suite extension.}
If additional experiments are available, we report the same training-objective and input ablations
across all LIBERO suites in Table~\ref{tab:selector_training_ablation_all_suites}. Otherwise, the
main ablation is reported on LIBERO-Object, where all three injected failure types are balanced and
the selector gains are most directly comparable to the main analysis.

\begin{table}[t]
\centering
\caption{
Optional all-suite selector training ablation. Fill this table if the same ablation is run beyond
LIBERO-Object.
}
\label{tab:selector_training_ablation_all_suites}
\begin{tabular}{lccccc}
\toprule
Variant & Object & Spatial & Goal & Long & Avg. \\
\midrule
Scratch sup. & [fill] & [fill] & [fill] & [fill] & [fill] \\
Proxy sup. & [fill] & [fill] & [fill] & [fill] & [fill] \\
Weak RL & [fill] & [fill] & [fill] & [fill] & [fill] \\
RL + Pos. BC & [fill] & [fill] & [fill] & [fill] & [fill] \\
B2FF & [fill] & [fill] & [fill] & [fill] & [fill] \\
\bottomrule
\end{tabular}
\end{table}
%%%%%%%%%%%%%%%%%%%%%%%%%%%%%%%%%%%%%%%%%%%
\section{Failure-Injected LIBERO Benchmark}
\label{app:failure_injected_libero}

\subsection{Benchmark Construction Overview}
\label{app:benchmark_construction}

Standard LIBERO evaluates task completion from a clean initial state without externally injected
perturbations. Failure-injected LIBERO instead introduces a controlled off-trajectory deviation
during policy execution. Starting from the same task and initial-state distribution, we first execute
the frozen VLA under nominal control and then inject a single perturbation at a randomly sampled
failure time $t_{\mathrm{fail}}$. After the perturbation, we compare recovery strategies such as no-fix
execution, fixed milestone rules, visual-nearest selection, and the recoverability-aware B2FF
selector.

For selector training, we construct offline counterfactual recovery groups. Each group shares the
same failure context, including the same task, initial state, perturbation type, perturbation parameters,
and failure observation. For this shared context, we clamp different candidate familiar milestones
and roll out the frozen VLA to obtain candidate-wise success labels. These counterfactual rollouts
are used only for selector training and candidate-oracle analysis. At test time, B2FF performs a
single selector forward pass and does not perform candidate-wise trial rollouts.
%%%%%%%%%%%%%%%%%%%%%%%%%%%%%%%%%%%%%%%%%%%%%
\subsection{Failure Type Definitions}
\label{app:failure_type_definitions}

We consider three families of recoverable perturbations.

\paragraph{Gripper XY offset.}
This perturbation models end-effector misalignment. We sample a random direction in the XY plane
and apply a bounded offset from the current end-effector position using a short controller sequence.
This intentionally moves the gripper away from the nominal interaction pose while keeping the task
physically recoverable.

\paragraph{Object XY shift.}
This perturbation models target-object displacement. We directly modify the XY position of the
target or goal object's MuJoCo joint pose. The displacement direction is sampled as a random XY
direction. Unless explicitly overridden, we do not apply yaw jitter in the final runs. This creates a
state where the object has moved away from the nominal trajectory but remains within the workspace.

\paragraph{Object laydown.}
This perturbation models an unexpected object pose or orientation change. We multiply the object's
free-joint quaternion by an X-axis or Y-axis tilt rotation, causing the object to enter a laid-down or
otherwise unexpected stable orientation. When needed, the object is slightly lifted before the pose
change to avoid invalid contact during perturbation.
%%%%%%%%%%%%%%%%%%%%%%%%%%%%%%%%%%%%%%%%%%%%%%
\subsection{Perturbation Ranges}
\label{app:perturbation_ranges}

Table~\ref{tab:failure_injection_specs} summarizes the perturbation ranges used in
failure-injected LIBERO. Gripper and object shifts are sampled in the XY plane. Object laydown
perturbations are sampled by choosing an X-axis or Y-axis tilt and applying the corresponding
orientation change to the object free joint. All perturbations are bounded so that the task remains
physically plausible and the relevant object remains observable and reachable.

\begin{table}[t]
\centering
\caption{
Failure-injection specifications. Each failure-injected episode contains one perturbation sampled
from the listed ranges.
}
\label{tab:failure_injection_specs}
\begin{tabular}{llll}
\toprule
Failure type & Affected entity & Perturbation range & Additional details \\
\midrule
Gripper XY offset
& End-effector
& Small: 4--6 cm; medium: 6--8 cm; large: 8--10 cm
& Random XY direction \\

Object XY shift
& Target / goal object
& Small: 1--2 cm; medium: 3--4 cm; large: 5--6 cm
& Random XY direction; MuJoCo joint pose; yaw jitter $0^\circ$ by default \\

Object laydown
& Target / goal object
& Tilt: 70--85$^\circ$ or 85--100$^\circ$
& X or Y axis; yaw $0^\circ$ by default; lift 0.8 cm \\
\bottomrule
\end{tabular}
\end{table}
%%%%%%%%%%%%%%%%%%%%%%%%%%%%%%%%%%%%%%%%%%%%%%%
\subsection{Injection Timing}
\label{app:injection_timing}

Each failure-injected episode contains one perturbation applied at a randomly sampled failure time
$t_{\mathrm{fail}}$. The sampling range is chosen so that the perturbation occurs during meaningful
task execution rather than immediately after reset or after the episode is effectively over. Most
perturbations occur before grasp or before stable object placement. When a perturbation occurs
after grasp, it simulates a bounded slip-or-drop-like deviation while still preserving a recoverable
task state.

Table~\ref{tab:failure_timing_bins} reports the timing-bin distribution. Timing bins are measured
in environment steps. The training row reports the 400 offline counterfactual recovery groups used
for selector training, while the evaluation row reports the 480 held-out failure-injected evaluation
episodes.

\begin{table}[t]
\centering
\caption{
Failure-injection timing distribution. Timing bins are reported in environment steps. Counts should
sum to 400 for selector-training groups and 480 for held-out evaluation episodes.
}
\label{tab:failure_timing_bins}
\begin{tabular}{lcccccc}
\toprule
Split & 40--49 & 50--59 & 60--69 & 70--79 & 80--90 & Total \\
\midrule
Selector training groups & [fill] & [fill] & [fill] & [fill] & [fill] & 400 \\
Evaluation episodes      & [fill] & [fill] & [fill] & [fill] & [fill] & 480 \\
\bottomrule
\end{tabular}
\end{table}

In controlled recovery evaluation, B2FF enters recovery mode at the injected perturbation time in
order to isolate the effect of milestone selection. In the online-triggered variant, the recovery entry
time is estimated from proprioceptive history instead.
%%%%%%%%%%%%%%%%%%%%%%%%%%%%%%%%%%%%%%%%%%
\subsection{Recoverability and Exclusion Criteria}
\label{app:recoverability_exclusion}

Failure-injected LIBERO is designed to evaluate recovery from bounded, physically plausible
off-trajectory deviations. We restrict perturbation magnitudes so that the relevant object generally
remains inside the workspace, observable from the policy cameras, and reachable by the robot.
Perturbations are skipped when the failure cannot be triggered, when the simulation enters an invalid
state, or when no valid familiar milestone bank can be constructed.

We do not claim to cover arbitrary irreversible failures. The benchmark focuses on recoverable
deviations such as end-effector misalignment, nearby object displacement, and unexpected but still
feasible object pose changes. Failures such as missing objects, severe occlusions, workspace exits,
unachievable instructions, or skills absent from the underlying VLA are outside the scope of this
benchmark.
%%%%%%%%%%%%%%%%%%%%%%%%%%%%%%%%%%%%%%%%%%%%%
\subsection{Dataset Splits and Episode Counts}
\label{app:dataset_splits_counts}

We use 400 offline counterfactual recovery groups for selector training. These groups are used to
train the recoverability-aware selector from candidate-wise recovery outcomes.

For failure-injected evaluation, we construct a held-out evaluation set of 480 episodes across four
LIBERO suites. Each suite contains 120 episodes, balanced across the three failure types: 40 gripper
XY offset episodes, 40 object XY shift episodes, and 40 object laydown episodes.

\begin{table}[t]
\centering
\caption{
Failure-injected LIBERO evaluation episodes by suite and failure type. Each suite contains
120 episodes, balanced as 40/40/40 across the three injected failure types.
}
\label{tab:failure_injected_eval_counts}
\begin{tabular}{lcccc}
\toprule
Suite & Gripper XY offset & Object XY shift & Object laydown & Total \\
\midrule
LIBERO-Object  & 40 & 40 & 40 & 120 \\
LIBERO-Spatial & 40 & 40 & 40 & 120 \\
LIBERO-Goal    & 40 & 40 & 40 & 120 \\
LIBERO-Long    & 40 & 40 & 40 & 120 \\
\midrule
Total          & 160 & 160 & 160 & 480 \\
\bottomrule
\end{tabular}
\end{table}

All methods are evaluated on the same held-out failure-injected episodes. For each episode, the
task, initial state, language instruction, failure type, perturbation parameters, and injection time are
fixed across methods.
%%%%%%%%%%%%%%%%%%%%%%%%%%%%%%%%%%%%%%%%%%%%%%%
\subsection{Evaluation Protocol}
\label{app:evaluation_protocol}

Each failure-injected rollout contains one perturbation. After environment reset, we execute a
10-step warm-up phase before the actual rollout begins. This stabilizes the simulator, renderer, and
controller state before policy execution.

Unless otherwise stated, we use action chunks of length 10, a familiar future bank initialized with
12 milestones, candidate offsets $\Delta=\{-1,0,+1,+2,+4\}$, and a selector history window of
4 observations. For offline counterfactual candidate collection, the default recovery horizon is
5 decision steps. Final task success is measured using the standard LIBERO task-success condition.

During controlled evaluation, the recovery trigger is aligned with $t_{\mathrm{fail}}$ to isolate
milestone selection. During online-triggered evaluation, recovery timing is estimated from
proprioceptive history. At test time, B2FF selects one milestone $v^\star$, fixes it as the
future-image subgoal, and executes the frozen VLA in action-only denoising mode.
%%%%%%%%%%%%%%%%%%%%%%%%%%%%%%%%%%%%%%%%%%

\section{Baselines and Selection Rules}
\label{app:baselines_selection_rules}

\subsection{Shared Recovery Protocol}
\label{app:shared_recovery_protocol}

For B2FF-specific comparisons, we keep the frozen VLA, familiar future bank, recovery entry time,
candidate offset set, and recovery window fixed across methods. The methods differ only in which
future visual condition is used after recovery begins. In controlled failure-injected evaluation, all
methods enter recovery at the same perturbation-aligned index $f$. In the online-triggered variant,
the entry time is estimated by the learned detector, but the same selection rule definitions apply once
recovery begins.

Given the familiar future bank $B$ and local candidate set $C_f$, a selection rule chooses either a
candidate milestone $v^\star\in C_f$ or a newly re-predicted failed-state future. The chosen visual
condition is then used by the frozen VLA during the recovery window. No selection-rule baseline
updates the VLA weights.
%%%%%%%%%%%%%%%%%%%%%%%%%%%%%%%%%%%%%%%
\subsection{Base VLA and Failed-State Re-Planning}
\label{app:udvla_failed_state_replan}

\paragraph{UD-VLA / no-fix baseline.}
The base UD-VLA policy is the frozen foresight-driven VLA used by B2FF. It runs in the nominal
joint subgoal--action generation mode throughout the episode:
\[
    (\hat v_t,a_t)\sim \pi_\theta(v,a\mid I,o_t).
\]
After an injected failure, this baseline does not explicitly enter a recovery mode, does not use the
familiar future bank, and does not invoke the B2FF selector. It simply continues querying the
frozen VLA from the current observation.

\paragraph{Failed-state re-planning.}
Failed-state re-planning is the recovery-time analogue of the base VLA response to an
off-trajectory observation. When recovery begins at failure observation $o_f$, the policy directly
re-predicts a new future and action from the failed state:
\[
    (\hat v_f,a_f)\sim \pi_\theta(v,a\mid I,o_f).
\]
This baseline tests whether the VLA can recover by re-imagining the future from the unfamiliar
failure observation itself. In contrast, B2FF avoids re-predicting the recovery future from $o_f$ and
instead selects a pre-imagined familiar milestone from the bank constructed before execution.
%%%%%%%%%%%%%%%%%%%%%%%%%%%%%%%%%%%%%%%%%%
\subsection{Fixed-Anchor Baselines}
\label{app:fixed_anchor_baselines}

Fixed-anchor baselines choose a milestone using a hand-designed progress rule rather than a
learned recoverability score. Let $f$ be the recovery entry index. We evaluate the following fixed
rules:
\[
\begin{aligned}
    \textsc{Fixed-Previous}:&\quad v^\star=\tilde v_{f-1},\\
    \textsc{Fixed-Current}:&\quad v^\star=\tilde v_{f},\\
    \textsc{Fixed-Near}:&\quad v^\star=\tilde v_{f+1}.
\end{aligned}
\]
If the requested index is outside the valid bank range, we use the closest valid candidate in $C_f$.
After choosing the fixed anchor, the method uses the same action-only denoising recovery mode as
B2FF:
\[
    a_t\sim \pi_\theta(a\mid I,o_t;\;v_t\leftarrow v^\star).
\]

We also report \textsc{Best-Fixed}, which is the strongest aggregate result among
\textsc{Fixed-Previous}, \textsc{Fixed-Current}, and \textsc{Fixed-Near}. This is not a per-episode
oracle and does not select the best fixed rule separately for each failure instance; it is only a summary
of the best fixed-anchor baseline at the reported evaluation level.
%%%%%%%%%%%%%%%%%%%%%%%%%%%%%%%%%%%%%%
\subsection{Visual-Nearest Baseline}
\label{app:visual_nearest_baseline}

The visual-nearest baseline selects the candidate milestone that is most visually similar to the
failure observation in the frozen visual-tokenizer feature space. Let $E_{\mathrm{vis}}$ denote the
frozen visual tokenizer and let
\[
    z(x)=\mathrm{Normalize}(\mathrm{Pool}(E_{\mathrm{vis}}(x)))
\]
be the pooled and normalized visual feature for image $x$. The visual-nearest baseline chooses
\[
    v^\star
    =
    \arg\max_{\tilde v\in C_f}
    z(o_f)^\top z(\tilde v).
\]
This baseline uses no recovery labels and no learned selector. It tests whether visual similarity to
the failed observation is sufficient for selecting a useful recovery milestone. Since a recoverable
future anchor need not pixel-match the failed observation, visual-nearest can choose candidates that
look similar but do not provide a good action-guiding condition.
%%%%%%%%%%%%%%%%%%%%%%%%%%%%%%%%%%%%%%%
\subsection{Recoverability-Aware B2FF Selector}
\label{app:b2ff_selection_rule}

B2FF uses the learned selector $F_\phi$ to choose the milestone that is predicted to be most
recoverable from the current failure context. Given failure observation $o_f$, recent history $H_f$,
and local candidate set $C_f$, B2FF selects
\[
    v^\star
    =
    \arg\max_{\tilde v\in C_f}
    F_\phi(\tilde v\mid o_f,H_f,C_f).
\]
The selector is evaluated with a single forward pass at test time. It does not perform candidate-wise
trial rollouts. Once selected, $v^\star$ is fixed as the future-image subgoal for the recovery window.
%%%%%%%%%%%%%%%%%%%%%%%%%%%%%%%%%%%%%
\subsection{Recoverability-Aware B2FF Selector}
\label{app:b2ff_selection_rule}

B2FF uses the learned selector $F_\phi$ to choose the milestone that is predicted to be most
recoverable from the current failure context. Given failure observation $o_f$, recent history $H_f$,
and local candidate set $C_f$, B2FF selects
\[
    v^\star
    =
    \arg\max_{\tilde v\in C_f}
    F_\phi(\tilde v\mid o_f,H_f,C_f).
\]
The selector is evaluated with a single forward pass at test time. It does not perform candidate-wise
trial rollouts. Once selected, $v^\star$ is fixed as the future-image subgoal for the recovery window.
%%%%%%%%%%%%%%%%%%%%%%%%%%%%%%%%%%%%%%%%%%
\subsection{Summary of Selection Rules}
\label{app:selection_rule_summary}

\begin{table}[t]
\centering
\caption{
Summary of recovery-time selection rules. All B2FF-specific variants use the same frozen VLA and
the same recovery entry point; they differ only in the visual condition used during recovery.
}
\label{tab:selection_rule_summary}
\begin{tabular}{llll}
\toprule
Method & Recovery visual condition & Uses bank? & Uses test-time rollouts? \\
\midrule
UD-VLA / no-fix
& Re-predicted by $\pi_\theta(v,a\mid I,o_t)$
& No
& No \\

Failed-state re-plan
& Future re-predicted from $o_f$
& No
& No \\

Fixed-Previous
& $\tilde v_{f-1}$
& Yes
& No \\

Fixed-Current
& $\tilde v_f$
& Yes
& No \\

Fixed-Near
& $\tilde v_{f+1}$
& Yes
& No \\

Visual-nearest
& $\arg\max_{\tilde v\in C_f} z(o_f)^\top z(\tilde v)$
& Yes
& No \\

B2FF
& $\arg\max_{\tilde v\in C_f} F_\phi(\tilde v\mid o_f,H_f,C_f)$
& Yes
& No \\

Candidate oracle
& Any successful candidate in $C_f$
& Yes
& Yes, offline only \\
\bottomrule
\end{tabular}
\end{table}
\subsection{Comparison to Action-Level Correction Methods}

\section{Protocol Ablations}
\subsection{Bank Size}
\subsection{Candidate Offsets}
\subsection{Recovery Window Length}
\subsection{Trigger Timing}
\subsection{Action Chunk Length and Bank-Index Mapping}

\section{Full Simulation Results}
\label{app:full_sim_results}

\newcommand{\emptycell}{--}

This section provides the full simulation results omitted from the main paper for space. We report
failure-injected LIBERO results by suite and failure type, standard LIBERO results by suite and task,
per-task gains and regressions, and selector score calibration.

\subsection{Failure-Injected LIBERO Results}
\label{app:failure_injected_full_results}

Table~\ref{tab:failure_injected_full} reports the full failure-injected LIBERO results. Each suite is
evaluated under three injected failure types: gripper shift, object shift, and object laydown. Unless
otherwise noted, success rates are final task success rates in percent. The average column is computed
over all suite--failure-type cells. Confidence intervals are computed over evaluation episodes.

\begin{table*}[t]
\centering
\scriptsize
\caption{
Full failure-injected LIBERO results by suite and injected failure type. Values are final task success
rates (\%). ``Grip.'' denotes gripper shift, ``Shift'' denotes object shift, and ``Lay.'' denotes object
laydown. Fill in $N$ and confidence intervals using the final evaluation logs.
}
\label{tab:failure_injected_full}
\resizebox{\linewidth}{!}{
\begin{tabular}{lccccccccccccccc}
\toprule
Method
& \multicolumn{3}{c}{Object}
& \multicolumn{3}{c}{Spatial}
& \multicolumn{3}{c}{Goal}
& \multicolumn{3}{c}{Long}
& Avg. & $N$ & 95\% CI \\
\cmidrule(lr){2-4}
\cmidrule(lr){5-7}
\cmidrule(lr){8-10}
\cmidrule(lr){11-13}
& Grip. & Shift & Lay.
& Grip. & Shift & Lay.
& Grip. & Shift & Lay.
& Grip. & Shift & Lay.
& & & \\
\midrule
DP
& \emptycell & \emptycell & \emptycell
& \emptycell & \emptycell & \emptycell
& \emptycell & \emptycell & \emptycell
& \emptycell & \emptycell & \emptycell
& \emptycell & \emptycell & \emptycell \\
DCDP
& \emptycell & \emptycell & \emptycell
& \emptycell & \emptycell & \emptycell
& \emptycell & \emptycell & \emptycell
& \emptycell & \emptycell & \emptycell
& \emptycell & \emptycell & \emptycell \\
MolmoAct
& \emptycell & \emptycell & \emptycell
& \emptycell & \emptycell & \emptycell
& \emptycell & \emptycell & \emptycell
& \emptycell & \emptycell & \emptycell
& \emptycell & \emptycell & \emptycell \\
SPR-VLA
& \emptycell & \emptycell & \emptycell
& \emptycell & \emptycell & \emptycell
& \emptycell & \emptycell & \emptycell
& \emptycell & \emptycell & \emptycell
& \emptycell & \emptycell & \emptycell \\
UD-VLA
& \emptycell & \emptycell & \emptycell
& \emptycell & \emptycell & \emptycell
& \emptycell & \emptycell & \emptycell
& \emptycell & \emptycell & \emptycell
& \emptycell & \emptycell & \emptycell \\
B2FF
& \emptycell & \emptycell & \emptycell
& \emptycell & \emptycell & \emptycell
& \emptycell & \emptycell & \emptycell
& \emptycell & \emptycell & \emptycell
& \emptycell & \emptycell & \emptycell \\
B2FF (online trigger)
& \emptycell & \emptycell & \emptycell
& \emptycell & \emptycell & \emptycell
& \emptycell & \emptycell & \emptycell
& \emptycell & \emptycell & \emptycell
& \emptycell & \emptycell & \emptycell \\
\bottomrule
\end{tabular}
}
\end{table*}
\subsection{Standard LIBERO Results}
\label{app:standard_libero_full_results}

Table~\ref{tab:standard_libero_suite_full} reports suite-level results on standard LIBERO, where no
external perturbation is injected. In addition to final success rate, we report how often B2FF enters
recovery mode during standard rollouts. This helps verify whether the recovery interface improves
naturally occurring deviations without unnecessarily perturbing successful nominal rollouts.

\begin{table}[t]
\centering
\scriptsize
\caption{
Standard LIBERO suite-level results. Values are final task success rates (\%) unless otherwise noted.
Trigger rate is the fraction of standard rollouts in which B2FF enters recovery mode.
}
\label{tab:standard_libero_suite_full}
\resizebox{\linewidth}{!}{
\begin{tabular}{lcccccccc}
\toprule
Method
& Object & Spatial & Goal & Long & Avg.
& $N$
& Trigger rate
& No-trigger success \\
\midrule
DP
& \emptycell & \emptycell & \emptycell & \emptycell & \emptycell
& \emptycell & \emptycell & \emptycell \\
DCDP
& \emptycell & \emptycell & \emptycell & \emptycell & \emptycell
& \emptycell & \emptycell & \emptycell \\
MolmoAct
& \emptycell & \emptycell & \emptycell & \emptycell & \emptycell
& \emptycell & \emptycell & \emptycell \\
SPR-VLA
& \emptycell & \emptycell & \emptycell & \emptycell & \emptycell
& \emptycell & \emptycell & \emptycell \\
UD-VLA
& \emptycell & \emptycell & \emptycell & \emptycell & \emptycell
& \emptycell & \emptycell & \emptycell \\
B2FF
& \emptycell & \emptycell & \emptycell & \emptycell & \emptycell
& \emptycell & \emptycell & \emptycell \\
B2FF (online trigger)
& \emptycell & \emptycell & \emptycell & \emptycell & \emptycell
& \emptycell & \emptycell & \emptycell \\
\bottomrule
\end{tabular}
}
\end{table}

\begin{table}[t]
\centering
\scriptsize
\caption{
Trigger statistics on standard LIBERO. This table separates triggered and non-triggered rollouts to
check whether B2FF leaves successful nominal executions unaffected.
}
\label{tab:standard_trigger_stats}
\resizebox{\linewidth}{!}{
\begin{tabular}{lcccccc}
\toprule
Suite
& $N$
& Triggered episodes
& Trigger rate
& Success without trigger
& Success with trigger
& Success change on no-trigger episodes \\
\midrule
Object  & \emptycell & \emptycell & \emptycell & \emptycell & \emptycell & \emptycell \\
Spatial & \emptycell & \emptycell & \emptycell & \emptycell & \emptycell & \emptycell \\
Goal    & \emptycell & \emptycell & \emptycell & \emptycell & \emptycell & \emptycell \\
Long    & \emptycell & \emptycell & \emptycell & \emptycell & \emptycell & \emptycell \\
All     & \emptycell & \emptycell & \emptycell & \emptycell & \emptycell & \emptycell \\
\bottomrule
\end{tabular}
}
\end{table}

\subsection{Per-Task Results}
\label{app:per_task_results}

Table~\ref{tab:standard_per_task} reports per-task standard LIBERO results. We include the task
instruction when space permits, the baseline success rate, B2FF success rate, and the absolute
change in success rate. Table~\ref{tab:failure_injected_per_task} provides the corresponding
per-task failure-injected results.

\begin{longtable}{llp{0.36\linewidth}cccccc}
\caption{
Standard LIBERO per-task results. Values are final task success rates (\%). $\Delta$ denotes
B2FF minus UD-VLA.
}
\label{tab:standard_per_task}
\\
\toprule
Suite & Task ID & Language instruction
& $N$
& UD-VLA
& B2FF
& B2FF online
& $\Delta$
& Trigger rate \\
\midrule
\endfirsthead

\toprule
Suite & Task ID & Language instruction
& $N$
& UD-VLA
& B2FF
& B2FF online
& $\Delta$
& Trigger rate \\
\midrule
\endhead

Object  & \emptycell & \emptycell & \emptycell & \emptycell & \emptycell & \emptycell & \emptycell & \emptycell \\
Object  & \emptycell & \emptycell & \emptycell & \emptycell & \emptycell & \emptycell & \emptycell & \emptycell \\
Spatial & \emptycell & \emptycell & \emptycell & \emptycell & \emptycell & \emptycell & \emptycell & \emptycell \\
Spatial & \emptycell & \emptycell & \emptycell & \emptycell & \emptycell & \emptycell & \emptycell & \emptycell \\
Goal    & \emptycell & \emptycell & \emptycell & \emptycell & \emptycell & \emptycell & \emptycell & \emptycell \\
Goal    & \emptycell & \emptycell & \emptycell & \emptycell & \emptycell & \emptycell & \emptycell & \emptycell \\
Long    & \emptycell & \emptycell & \emptycell & \emptycell & \emptycell & \emptycell & \emptycell & \emptycell \\
Long    & \emptycell & \emptycell & \emptycell & \emptycell & \emptycell & \emptycell & \emptycell & \emptycell \\

\bottomrule
\end{longtable}

\begin{longtable}{llp{0.30\linewidth}ccccccc}
\caption{
Failure-injected LIBERO per-task results. Values are final task success rates (\%). The failure-type
columns report B2FF success rate under each injected failure type.
}
\label{tab:failure_injected_per_task}
\\
\toprule
Suite & Task ID & Language instruction
& $N$
& UD-VLA
& B2FF
& $\Delta$
& Grip.
& Shift
& Lay. \\
\midrule
\endfirsthead

\toprule
Suite & Task ID & Language instruction
& $N$
& UD-VLA
& B2FF
& $\Delta$
& Grip.
& Shift
& Lay. \\
\midrule
\endhead

Object  & \emptycell & \emptycell & \emptycell & \emptycell & \emptycell & \emptycell & \emptycell & \emptycell & \emptycell \\
Object  & \emptycell & \emptycell & \emptycell & \emptycell & \emptycell & \emptycell & \emptycell & \emptycell & \emptycell \\
Spatial & \emptycell & \emptycell & \emptycell & \emptycell & \emptycell & \emptycell & \emptycell & \emptycell & \emptycell \\
Spatial & \emptycell & \emptycell & \emptycell & \emptycell & \emptycell & \emptycell & \emptycell & \emptycell & \emptycell \\
Goal    & \emptycell & \emptycell & \emptycell & \emptycell & \emptycell & \emptycell & \emptycell & \emptycell & \emptycell \\
Goal    & \emptycell & \emptycell & \emptycell & \emptycell & \emptycell & \emptycell & \emptycell & \emptycell & \emptycell \\
Long    & \emptycell & \emptycell & \emptycell & \emptycell & \emptycell & \emptycell & \emptycell & \emptycell & \emptycell \\
Long    & \emptycell & \emptycell & \emptycell & \emptycell & \emptycell & \emptycell & \emptycell & \emptycell & \emptycell \\

\bottomrule
\end{longtable}

\subsection{Largest Per-Task Gains and Regressions}
\label{app:task_gains_regressions}

To make the per-task results easier to interpret, we separately list the tasks where B2FF improves
most over the base VLA and the tasks where B2FF underperforms the base VLA.

\begin{table}[t]
\centering
\scriptsize
\caption{
Tasks with the largest B2FF gains over UD-VLA. $\Delta$ denotes B2FF minus UD-VLA.
}
\label{tab:largest_task_gains}
\resizebox{\linewidth}{!}{
\begin{tabular}{cllp{0.40\linewidth}cccc}
\toprule
Rank & Suite & Task ID & Language instruction
& $N$ & UD-VLA & B2FF & $\Delta$ \\
\midrule
1 & \emptycell & \emptycell & \emptycell & \emptycell & \emptycell & \emptycell & \emptycell \\
2 & \emptycell & \emptycell & \emptycell & \emptycell & \emptycell & \emptycell & \emptycell \\
3 & \emptycell & \emptycell & \emptycell & \emptycell & \emptycell & \emptycell & \emptycell \\
4 & \emptycell & \emptycell & \emptycell & \emptycell & \emptycell & \emptycell & \emptycell \\
5 & \emptycell & \emptycell & \emptycell & \emptycell & \emptycell & \emptycell & \emptycell \\
\bottomrule
\end{tabular}
}
\end{table}

\begin{table}[t]
\centering
\scriptsize
\caption{
Tasks where B2FF underperforms UD-VLA. Negative $\Delta$ indicates a regression relative to the
base VLA.
}
\label{tab:largest_task_regressions}
\resizebox{\linewidth}{!}{
\begin{tabular}{cllp{0.40\linewidth}cccc}
\toprule
Rank & Suite & Task ID & Language instruction
& $N$ & UD-VLA & B2FF & $\Delta$ \\
\midrule
1 & \emptycell & \emptycell & \emptycell & \emptycell & \emptycell & \emptycell & \emptycell \\
2 & \emptycell & \emptycell & \emptycell & \emptycell & \emptycell & \emptycell & \emptycell \\
3 & \emptycell & \emptycell & \emptycell & \emptycell & \emptycell & \emptycell & \emptycell \\
4 & \emptycell & \emptycell & \emptycell & \emptycell & \emptycell & \emptycell & \emptycell \\
5 & \emptycell & \emptycell & \emptycell & \emptycell & \emptycell & \emptycell & \emptycell \\
\bottomrule
\end{tabular}
}
\end{table}

\subsection{Selector Score Calibration}
\label{app:score_calibration}

We evaluate whether the selector scores are calibrated with respect to actual recovery success.
Following Fig.~\ref{fig:main_analysis}, we group candidate milestones into score quintiles and
measure the empirical success rate within each bin. A well-behaved selector should assign higher
scores to candidates that are more likely to recover the task.

\begin{table}[t]
\centering
\caption{
Selector score calibration on failure-injected LIBERO-Object. Candidates are grouped into
score quintiles. Success rate is the empirical fraction of candidates whose counterfactual rollout
succeeds.
}
\label{tab:score_calibration_quintiles}
\begin{tabular}{lccccc}
\toprule
Score bin
& Score range
& \# candidates
& \# successes
& Success rate
& 95\% CI \\
\midrule
Q1, lowest  & \emptycell & \emptycell & \emptycell & \emptycell & \emptycell \\
Q2          & \emptycell & \emptycell & \emptycell & \emptycell & \emptycell \\
Q3          & \emptycell & \emptycell & \emptycell & \emptycell & \emptycell \\
Q4          & \emptycell & \emptycell & \emptycell & \emptycell & \emptycell \\
Q5, highest & \emptycell & \emptycell & \emptycell & \emptycell & \emptycell \\
\bottomrule
\end{tabular}
\end{table}

\begin{table}[t]
\centering
\caption{
Selector reliability by selected-candidate score. This table evaluates calibration at the decision
level by binning the score of the candidate actually selected by B2FF in each recovery context.
}
\label{tab:selected_score_reliability}
\begin{tabular}{lccccc}
\toprule
Selected-score bin
& Score range
& \# recovery contexts
& \# successful recoveries
& Recovery success rate
& 95\% CI \\
\midrule
Q1, lowest  & \emptycell & \emptycell & \emptycell & \emptycell & \emptycell \\
Q2          & \emptycell & \emptycell & \emptycell & \emptycell & \emptycell \\
Q3          & \emptycell & \emptycell & \emptycell & \emptycell & \emptycell \\
Q4          & \emptycell & \emptycell & \emptycell & \emptycell & \emptycell \\
Q5, highest & \emptycell & \emptycell & \emptycell & \emptycell & \emptycell \\
\bottomrule
\end{tabular}
\end{table}

\section{Real-World Experiments}
\subsection{Robot Setup}
\subsection{Real-World Tasks}
\subsection{Demonstration Collection and VLA Training}
\subsection{Real-World Recovery Groups and Selector Tuning}
\subsection{Real-World Failure Injection}
\subsection{Full Real-World Breakdown}
\subsection{Selector-Training Overhead and Test-Time Latency}

\section{Qualitative Rollouts and Failure Cases}
\subsection{Additional Simulation Examples}
\subsection{Additional Real-World Examples}
\subsection{Failure Case Taxonomy}
\subsection{When Familiar Futures Help vs. Fail}

\section{Hyperparameters and Reproducibility Checklist}
\subsection{Main Hyperparameters}
\subsection{Compute Resources}
\subsection{Code-Level Details}
\subsection{Reproducibility Checklist}

% Optional
\section{Cross-Backbone Extension}
\subsection{Motivation}
\subsection{Target Backbone}
\subsection{Interface Mapping}
\subsection{Results}

\begin{table*}[t]
\centering
\scriptsize
\setlength{\tabcolsep}{2.8pt}

\resizebox{\textwidth}{!}{%
\begin{tabular}{@{}lrrrrrrrrrrrrrrrr@{}}
\toprule
& \multicolumn{4}{c}{\textbf{LIBERO-Object}}
& \multicolumn{4}{c}{\textbf{LIBERO-Spatial}}
& \multicolumn{4}{c}{\textbf{LIBERO-Goal}}
& \multicolumn{4}{c}{\textbf{LIBERO-Long}} \\
\cmidrule(lr){2-5}
\cmidrule(lr){6-9}
\cmidrule(lr){10-13}
\cmidrule(lr){14-17}
\textbf{Selection rule}
& \textbf{All} & \textbf{Grip.} & \textbf{Obj.} & \textbf{Lay.}
& \textbf{All} & \textbf{Grip.} & \textbf{Obj.} & \textbf{Lay.}
& \textbf{All} & \textbf{Grip.} & \textbf{Obj.} & \textbf{Lay.}
& \textbf{All} & \textbf{Grip.} & \textbf{Obj.} & \textbf{Lay.} \\
\midrule

\multicolumn{17}{@{}l}{\textsc{Nominal (no recovery)}} \\
Vanilla / no recovery
& \heat{52.5} & \heat{37.5} & \heat{52.5} & \heat{67.5}
& \heat{58.3} & \heat{75.0} & \heat{52.5} & \heat{47.5}
& \heat{58.3} & \heat{47.5} & \heat{60.0} & \heat{67.5}
& \heat{55.8} & \heat{62.5} & \heat{65.0} & \heat{40.0} \\
\midrule

\multicolumn{17}{@{}l}{\textsc{Heuristic baselines}} \\
Failed-state re-plan
& \heat{54.2} & \heat{47.5} & \heat{62.5} & \heat{52.5}
& \heat{51.7} & \heat{70.0} & \heat{52.5} & \heat{32.5}
& \heat{63.3} & \heat{62.5} & \heat{60.0} & \heat{67.5}
& \heat{69.2} & \heat{80.0} & \heat{75.0} & \heat{52.5} \\

Fixed previous
& \heat{50.8} & \heat{50.0} & \heat{55.0} & \heat{47.5}
& \heat{55.0} & \heat{82.5} & \heat{50.0} & \heat{32.5}
& \heat{60.0} & \heat{62.5} & \heat{57.5} & \heat{60.0}
& \heat{70.0} & \heat{70.0} & \heat{72.5} & \heat{67.5} \\

Fixed current
& \heat{57.5} & \heat{52.5} & \heat{52.5} & \heat{67.5}
& \heat{50.0} & \heat{70.0} & \heat{52.5} & \heat{27.5}
& \heat{58.3} & \heat{60.0} & \heat{55.0} & \heat{60.0}
& \heat{58.3} & \heat{57.5} & \heat{70.0} & \heat{47.5} \\

Fixed near
& \heat{30.8} & \heat{27.5} & \heat{37.5} & \heat{27.5}
& \heat{50.0} & \heat{75.0} & \heat{55.0} & \heat{20.0}
& \heat{55.0} & \heat{65.0} & \heat{60.0} & \heat{40.0}
& \heat{66.7} & \heat{85.0} & \heat{62.5} & \heat{52.5} \\

Random candidate
& \heat{49.2} & \heat{47.5} & \heat{50.0} & \heat{50.0}
& \heat{52.5} & \heat{77.5} & \heat{52.5} & \heat{27.5}
& \heat{59.2} & \heat{67.5} & \heat{60.0} & \heat{50.0}
& \heat{67.5} & \heat{75.0} & \heat{67.5} & \heat{60.0} \\

Visual nearest / heuristic
& \heat{50.8} & \heat{47.5} & \heat{52.5} & \heat{52.5}
& \heat{53.3} & \heat{75.0} & \heat{52.5} & \heat{32.5}
& \heat{59.2} & \heat{70.0} & \heat{60.0} & \heat{47.5}
& \heat{61.7} & \heat{72.5} & \heat{65.0} & \heat{47.5} \\

\arrayrulecolor{B2FFBlue}
\midrule
\rowcolor{B2FFBg}
\textbf{B2FF}
& \bhe{68.3} & \bhe{67.5} & \bhe{70.0} & \bhe{67.5}
& \bhe{62.5} & \bhe{92.5} & \bhe{55.0} & \bhe{40.0}
& \bhe{72.5} & \bhe{82.5} & \bhe{67.5} & \bhe{67.5}
& \bhe{83.3} & \bhe{100.0} & \bhe{82.5} & \bhe{67.5} \\
\midrule
\arrayrulecolor{black}

\multicolumn{17}{@{}l}{\textsc{Oracle (upper bound)}} \\
\rowcolor{OracleBg}
Candidate oracle
& \bocell{84.2} & \bocell{87.5} & \bocell{85.0} & \bocell{80.0}
& \bocell{69.2} & \bocell{95.0} & \bocell{65.0} & \bocell{47.5}
& \bocell{75.8} & \bocell{82.5} & \bocell{72.5} & \bocell{72.5}
& \bocell{85.0} & \bocell{100.0} & \bocell{82.5} & \bocell{72.5} \\

\bottomrule
\end{tabular}
}

\caption{
Familiar-future selection-rule ablation. Darker cells indicate higher success.
}
\label{tab:selection-rule-ablation}
\end{table*}
